# Supplementary material for: Physics at a 100 TeV pp collider: beyond the Standard Model phenomena
Source: arXiv:1606.00947 source file (2016-06-03)
Supplement: Supplementary file 7 [file declare.tex]

\newcommand\one{\leavevmode\hbox{\small1\normalsize\kern-.33em1}}

%\def\dslash{\not{\hbox{\kern-4pt $\partial$}}}
%\def\Dslash{\not{\hbox{\kern-4pt $D$}}}

%\newcommand{\mat}{\mathcal{M}}
%\newcommand{\slashed}[1]{\ensuremath{{#1}{\!}{\!}{\!}{\!}{\:}/}}

% all the masses 

% units of measure

% really great macro by Chris Lester
\def\slashchar#1{\setbox0=\hbox{$#1$}           % set a box for #1
   \dimen0=\wd0                                 % and get its size
   \setbox1=\hbox{/} \dimen1=\wd1               % get size of /
   \ifdim\dimen0>\dimen1                        % #1 is bigger
      \rlap{\hbox to \dimen0{\hfil/\hfil}}      % so center / in box
      #1                                        % and print #1
   \else                                        % / is bigger
      \rlap{\hbox to \dimen1{\hfil$#1$\hfil}}   % so center #1
      /                                         % and print /
   \fi}

%\DeclareMathOperator{\tr}{Tr}

% maximal number of floating environments on each page 
\setlength{\floatsep}{0pt}
\setcounter{topnumber}{1}
\setcounter{bottomnumber}{1}
\setcounter{totalnumber}{1}
